# Supplementary material for: c-axis pressure induced antiferromagnetic order in optimally P-doped BaFe2(As0.70P0.30)2 superconductor
Source: arXiv:1808.05153 source file (2018-08-15)
Supplement: Supplementary file 1 [file SI_2nd.pdf]

Supplementary Information

Single crystal sample preparation.

$BaFe_2(As_{0.70}P_{0.30})_2$ single crystals were grown with self-flux method as in our previous studies [1]. High quality crystals with flat surfaces were selected. The crystals were cut into 0.5*0.5 $mm^2$ squared shaped pieces with thickness of ~0.1 mm for transport measurements and 4*4 $mm^2$ pieces with thickness of ~0.4 mm for neutron scattering experiments.

Device for resistance measurements.

Uniaxial pressure was applied by our home-made device combined pneumatic pressure section with a feedback-controlled loop [2] and sample holder section [SFigure 1] in the resistance measurements. The sample was mounted in device and connected to standard PPMS sample puck by four-wire method with gold wires. We used sapphire as the substrate and attaching gold wires on the sample sides to make sure that the applied pressure is along the c-axis and homogeneous. Since our samples have large in-plane area but are thin for both neutron and transport measurements, we do not expect that the applied pressure will be vertical to the ab plane. As the smooth sapphire surface and the paper between sample and aluminum cylinder, the in-plane friction arising from differential thermal expansions in temperature changes will be tiny and negligible.

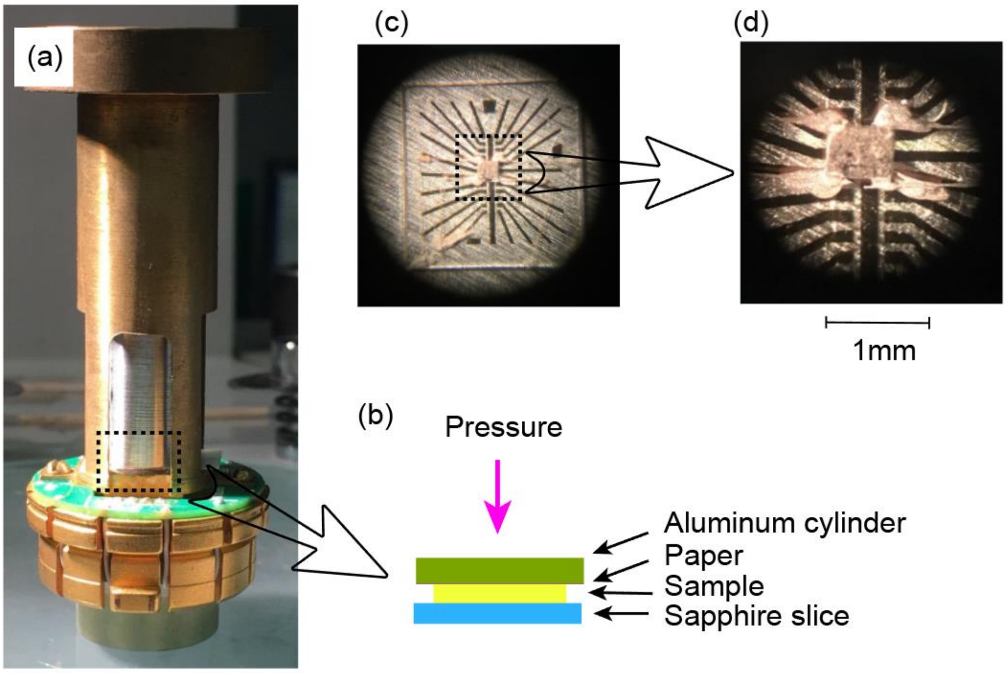


SFigure1: Sample holder section of pressure device, shown with sample mounted in the center of sapphire slice.

Device for neutron scattering experiment

The c-axis pressure device for neutron scattering experiments was made of 6601 aluminum alloy with low neutron incoherent scattering cross section. Uniaxial pressure was applied by compressing the stainless disc springs by hydraulic press and then fixed by the screw. No further change was made during the neutron scattering experiments. To distinguish the existence of effect from the friction and in-plane stress/strain between sample and aluminum plate in neutron scattering experiments, we have measured the magnetic order parameter on cooling and warming cycles. Negligible temperature hysteresis of magnetic order parameter has been found in our measurements.

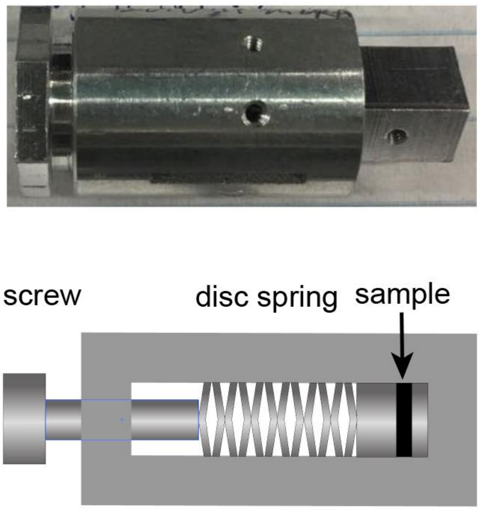


SFigure 2: Photo and schematic diagram of pressure cell used in neutron scattering experiment.

For experiments on HB-1A and MIRA, $BaFe_2(As_{0.70}P_{0.3})_2$ single crystal was aligned in the [1, 0, 0] x [0, 0, 1] scattering plane in orthorhombic notation. A PG filter on HB-1A and a Be-filter on MIRA were placed in the incident beam side to eliminate the influence from higher order neutrons.

At HB-3A, one single crystal mounted with pressure and another one without pressure were measured separately in two identical setup pressure cells. As the measurements were carried out at 295 K, we used the tetragonal notation. To obtain accurate information about the structural response to the c-axis uniaxial pressure, 30 unique Bragg peaks were measured for each case. The beam attenuation from the pressure cell was calculated for each reflection by measuring the same crystal with the pressure cell and without pressure cell both at ambient temperature. After applying the attenuation correction, the squared structure factors were obtained as listed in the Stable I and Stable II.

STable I. The squared structure factors of 30 measured reflections at T = 295 K ($\lambda_i$=1.546 Å, PG filter) with no pressure.

| *h* | *k* | *l* | $F^2$ | *error* | *h* | *k* | *l* | $F^2$ | *error* |
|---|---|---|---|---|---|---|---|---|---|
| 2 | 0 | 0 | 1238.23 | 32.83 | 0 | 2 | 0 | 1280.36 | 33.19 |

| | | | | | | | | | |
|---|---|---|---|---|---|---|---|---|---|
| 2 | 2 | 0 | 1280.33 | 37.66 | 0 | 0 | -10 | 1180.52 | 54.17 |
| 0 | 0 | -8 | 1364.15 | 56.85 | 0 | 0 | -6 | 45.73 | 10.98 |
| 0 | 0 | -4 | 390.51 | 22.94 | 0 | 0 | -2 | 526.98 | 19.01 |
| 1 | 0 | -1 | 13.32 | 5.66 | 1 | 0 | -3 | 572.13 | 27.34 |
| 1 | 1 | 0 | 6.87 | 6.57 | 1 | 1 | -2 | 833.90 | 29.79 |
| 1 | 0 | -5 | 74.85 | 13.52 | 1 | 1 | -4 | 1162.73 | 41.35 |
| 2 | 0 | -2 | 621.67 | 29.33 | 2 | 1 | -1 | 17.29 | 9.1 |
| 1 | 1 | -6 | 1998.98 | 61.18 | 2 | 0 | -4 | 378.45 | 28.59 |
| 1 | 0 | -7 | 85.12 | 16.46 | 2 | 1 | -3 | 561.04 | 29.86 |
| 2 | 1 | -5 | 65.39 | 15.40 | 2 | 0 | -6 | 48.35 | 14.81 |
| 2 | -2 | 0 | 1355.62 | 42.22 | 1 | 1 | -8 | 163.65 | 21.23 |
| 2 | 2 | -2 | 596.17 | 30.59 | 1 | 0 | -9 | 211.39 | 26.37 |
| 3 | 0 | -1 | 11.35 | 10.79 | 2 | 2 | -4 | 397.07 | 28.02 |
| 2 | 1 | -7 | 100.54 | 17.93 | 3 | 0 | -3 | 537.66 | 31.91 |

STable II. The squared structure factors of 30 measured reflections with pressure ($P = P_a$) at 295 K.

| *h* | *k* | *l* | $F^2$ | *error* | *h* | *k* | *l* | $F^2$ | *error* |
|---|---|---|---|---|---|---|---|---|---|
| 2 | 0 | 0 | 3156.99 | 34.08 | 0 | 2 | 0 | 3063.63 | 40.93 |
| 2 | 2 | 0 | 2854.55 | 32.81 | 0 | 0 | 10 | 1870.85 | 28.60 |
| 0 | 0 | 8 | 2193.61 | 58.91 | 0 | 0 | 6 | 91.55 | 17.54 |
| 0 | 0 | 4 | 453.81 | 20.67 | 0 | 0 | 2 | 739.62 | 34.49 |
| 1 | 0 | 1 | 14.11 | 2.41 | 1 | 0 | 3 | 840.83 | 43.84 |
| 1 | 1 | 0 | 12.29 | 2.38 | 1 | 1 | 2 | 1206.34 | 61.18 |
| 1 | 0 | 5 | 105.34 | 8.43 | 1 | 1 | 4 | 1526.99 | 66.47 |
| 2 | 0 | 2 | 860.90 | 39.96 | 2 | 1 | 1 | 13.47 | 2.69 |
| 1 | 1 | 6 | 2867.28 | 149.73 | 2 | 0 | 4 | 604.72 | 40.85 |
| 1 | 0 | 7 | 109.65 | 9.26 | 2 | 1 | 3 | 719.76 | 41.44 |
| 2 | 1 | 5 | 93.95 | 15.11 | 2 | 0 | 6 | 84.54 | 15.22 |
| 2 | 2 | 0 | 3024.43 | 97.39 | 1 | 1 | 8 | 203.86 | 18.24 |
| 2 | 2 | 2 | 768.52 | 33.43 | 1 | 0 | 9 | 296.93 | 16.51 |
| 3 | 0 | 1 | 11.29 | 2.90 | 2 | 2 | 4 | 580.41 | 28.70 |
| 2 | 1 | 7 | 95.38 | 9.28 | 3 | 0 | 3 | 682.52 | 24.96 |

## Magnetic DFT calculation results

| z(As,P) | | 0.349 | 0.3485 | 0.348 | 0.3475 | 0.347 |
|---|---|---|---|---|---|---|
| Δa/aexp=0 Δc/cexp=0 | GGA | 1.519 | 1.483 | 1.447 | 1.409 | 1.370 |
| | LSDA | 0.994 | 0.936 | 0.877 | 0.824 | 0.769 |
| Δa/aexp=0.5% | GGA | 1.541 | 1.507 | 1.472 | 1.436 | 1.400 |

| | | | | | | |
|---|---|---|---|---|---|---|
| Δc/cexp=-1% | LSDA | 0.967 | 0.914 | 0.859 | 0.804 | 0.752 |

STable III. The DFT-GGA/LSDA calculated Fe ordered magnetic moment (in unit of μB) in the stripe antiferromagnetic state as a function of As/P height z(As,P) using the experimental crystal structure and with 0.5% expanded experimental in-plane lattice constant and 1% compressed experimental c-lattice constant.

The magnetic DFT calculated Fe ordered magnetic moments in the stripe antiferromagnetic state are shown in STable III. First of all, the Fe magnetic moment remains finite in all the magnetic DFT calculations, therefore the experimental observation of the reemergence of the stripe antiferromagnetic states cannot be reproduced by magnetic DFT calculations using the popular GGA and LSDA exchange-correlation functionals. This is due to the well-known problem of GGA/LSDA of overestimating the Fe magnetic moment. Interestingly, the calculated Fe magnetic moment does increase with c-axis pressure. For example, at experimental lattice constants and z(As,P)=0.348, the GGA/LSDA Fe magnetic moment is 1.447/0.877 μB. With c-axis pressure, the in-plane lattice constant is expanded by 0.5%, the c-lattice constant is compressed by 1% and the z(As,P) =0.349 to keep the As/P height to Fe plane unchanged, the GGA/LSDA Fe magnetic moment becomes 1.541/0.967 μB, an increase of 0.094/0.09 μB, which has the same trend as DFT+DMFT calculations and experimental observation but overestimates the increased value, similar to the overestimation of the Fe magnetic moment.

References:

1. Hu., D. *et al.*, Phys. Rev. Lett. 114, 157002 (2015).
2. Tam., D. W., *et al.*, Phys. Rev. B 95, 060505(R) (2017).
